# Supplementary material for: Assignment-Control Plots: A Visual Companion for Causal Inference Study Design
Source: arXiv:2107.00122 source file (2021-06-30)
Supplement: Supplementary file 1 [file supplement.pdf]

# Supplementary Figures

## Assignment-Control Plots: A Visual Companion for Causal Inference Study Design

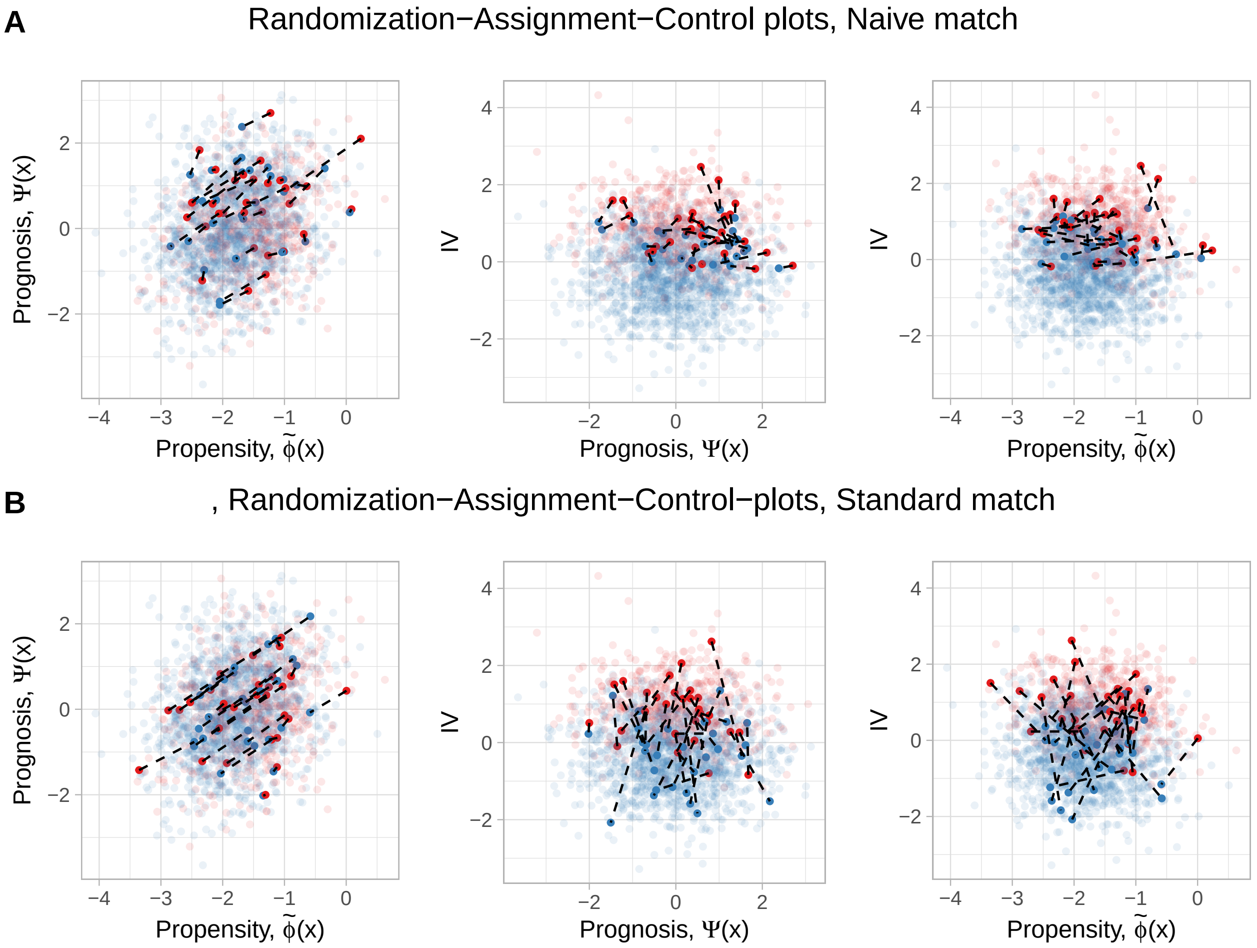


Figure 1: Randomization-Assignment-Control plots for two matching schemes. Data is generated according to the set-up in Figure 6 from the main text. In the naive match (A), observations are paired based on X1, X2 and Z, using Mahalanobis Distance. In the standard match (B), observations are paired based on X1, X2, and X3, where X3 is an uninformative covariate following the same marginal distribution as Z. When subjects are matched for nearness in the IV, randomizing variation within pairs is reduced, so the treated individual is more often the upper individual in the pair

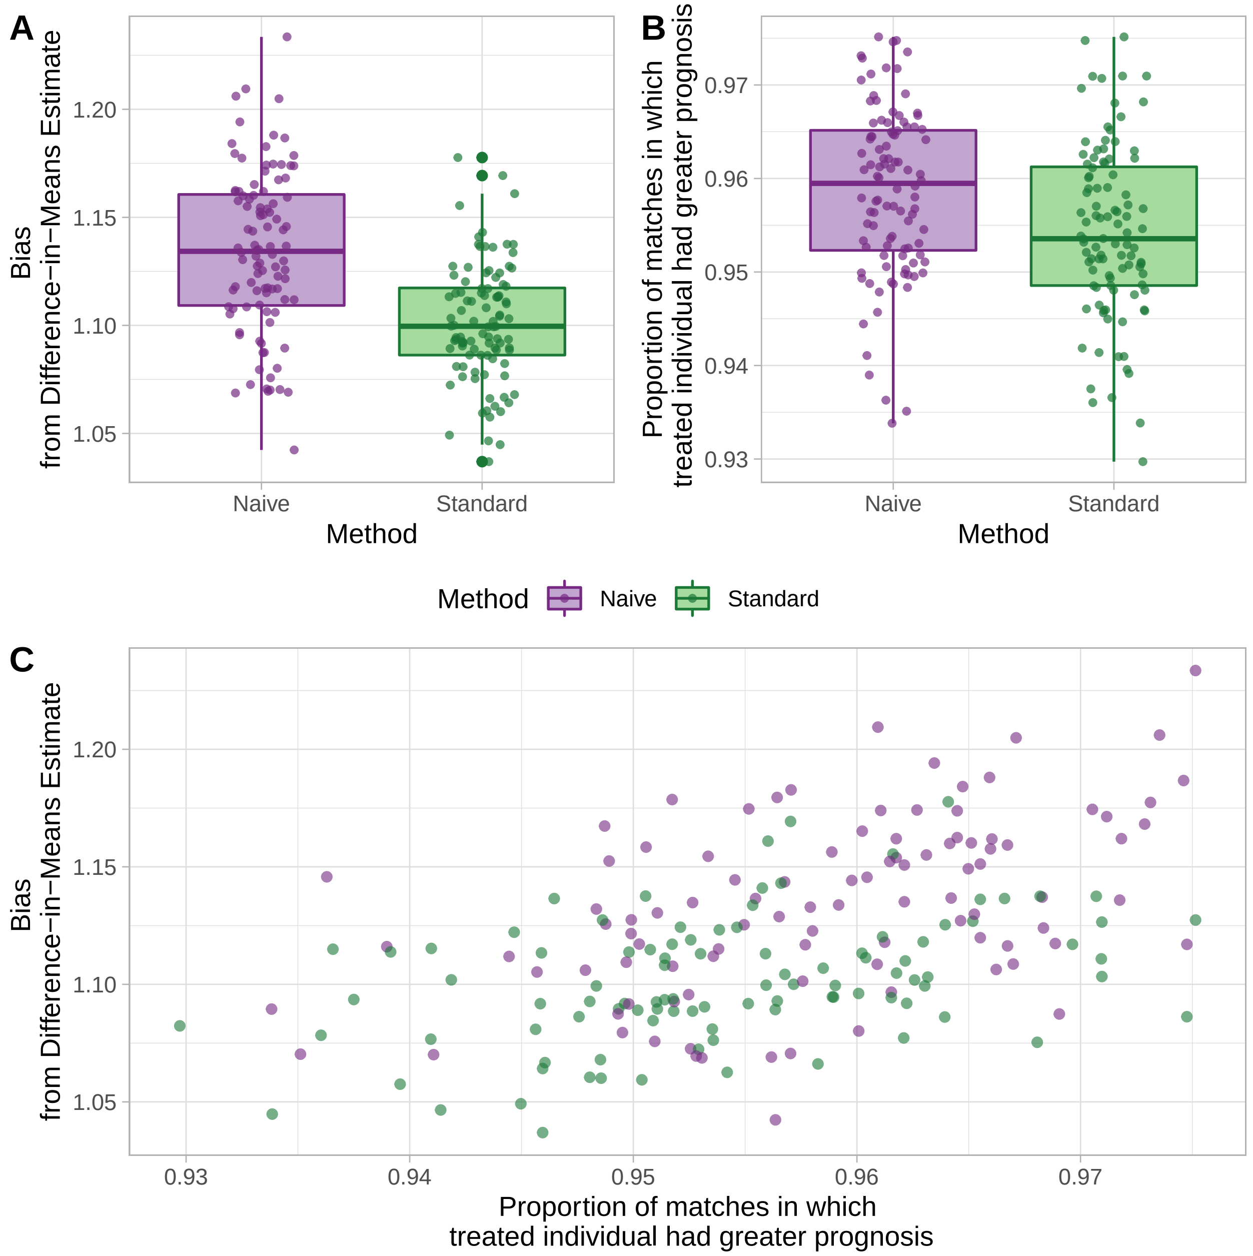


Figure 2: Simulation results (100 replicates) comparing two matching schemes in a scenario with an IV. Data is generated according to the set-up in Figure 6 from the main text, where Y(1) = Y(0) (i.e. there is no treatment effect). In the naive approach, observations are paired based on X1, X2 and Z, using Mahalanobis Distance. In the standard match, observations are paired based on X1, X2, and X3, where X3 is an uninformative covariate following the same marginal distribution as Z. The naive approach is more biased than the approach which excludes the IV from the matching (A), and in the naive approach, a greater proportion of matches select a treated individual with a higher expected Y(0) than the matched control (B). Matches in which a greater proportion of the matches select a treated individual with higher expected outcome than the matched control tend to be more biased (C).
